# Supplementary material for: Can Visual Context Improve Automatic Speech Recognition for an Embodied Agent?
Source: arXiv:2210.13189 source file (2022-10-21)
Supplement: Supplementary file 1 [file appendix.tex]

\section{Appendix}
\label{sec:appendix}
%This is a section, we provide a few detailed description that in the appendix.
\subsection{Acoustic modeling}
\label{sec:AM}
We use the Wav2Vec2~\cite{NEURIPS2020_92d1e1eb} for acoustic modeling of the speech. It transforms raw audio input into a contextual feature representation that can be further processed to predict labels from a sub-word level vocabulary - grapheme, phoneme or wordpiece. We have chosen grapheme units for a relatively simple algorithm design, but our approach is equally applicable to phoneme or wordpiece vocabulary. The model encodes raw audio waveform using several convolutional layers. The output of the final convolution layer is quantized and fed to a Transformer block that produces contextualized feature representation for the discrete time-steps $CF_1, \dots ,CF_L$, considering the entire sequence~\cite{NEURIPS2020_92d1e1eb}. The network is pre-trained in an self-supervised manner using 53.2k hours of unlabeled audio. To perform speech recognition, the pre-trained feature extractor $\textbf{CF}$ is fed to a linear layer with softmax and fine-tuned on annotated data from the LibriSpeech dataset~\cite{panayotov2015librispeech}, with the CTC loss function~\cite{graves2006connectionist}. The softmax produces a probability distribution over a character vocabulary in each time-step.
\subsection{Language model}
We use a 3-gram English language model\footnote{https://www.openslr.org/11/} trained on LibriSpeech data. More specifically, we use the \textit{3-gram.pruned.1e-7} variant of the language model in all of our experiments. We use the kenlm\footnote{https://github.com/kpu/kenlm} library for querying and calculating probabilities from language model. 
\subsection{Computing infrastructure \& runtime}
All of our experiments are performed in a laptop with an 11\textsuperscript{th} generation Intel i-5 processor with 2.6 GHz frequency, having 8 physical cores and 16 GB main memory. The operating system used was Ubuntu 20.04. We show the average run time decoding using our algorithm and different baselines in Table~\ref{tab:times}. Please note that because of the sampling function, a lesser number of candidates are generated in each time step, compared to the Base decoder. As a result, our decoding is actually faster. However, without sampling (which we do not advocate), an additional latency of (76.7-40.5)=36.2 ms on average is incurred for a single run.

\begin{table}[]
    \small
    \centering
    \begin{tabular}{|l|c|}
    \hline
         \textbf{Model}     &\textbf{Decoding time (ms)} \\ \hline
         Base   &   40.5 \\
         Base + LM  &51.5 \\
         Base + WB  &51.4 \\
         Base + WB \textsuperscript{ctx} &50.8 \\
         Ours, $C=1$    &76.7 \\
         Ours, $\sigma=0$   & 22.9 \\ 
         Ours           & 23.7 \\ \hline
    \end{tabular}
    \caption{Average decoding time per recording.}
    \label{tab:times}
\end{table}

\subsection{Validation results}
We report the WER and TA on the validation set in Table~\ref{tab:val-result}. These results are found by the separately optimized hyper-parameter search on the validation set.
\begin{table}[]
    \centering
    \small
    \begin{tabular}{|l|c|c|}
    \hline
    \textbf{Model}  &\textbf{WER} &\textbf{TA}\\ \hline
         Base   &13.49  & 65.1 \\
         Base + LM  & 13.23  & 66.1 \\
         Base + WB  & 10.27  & 74.6  \\
         Base + WB \textsuperscript{ctx} &10.14  & 75.6 \\
         Ours, $C=1$    & 10.34 & 79.4  \\
         Ours, $\sigma=0$   & 9.02  & 80.0  \\ 
         Ours           & 8.96  & 80.3 \\ \hline
    \end{tabular}
    \caption{Speech recognition results on validation set.}
    \label{tab:val-result}
\end{table}

\subsection{Hyper-parameters for other models}
We show the optimal hyper-parameters for all baselines and other variants of our model in Table~\ref{tab:hyper}. All models use beam width $N=100$.
The optimal hyper-parameters for our final model is shown in the main paper, in Table~\ref{tab:optimal-params}.
\begin{table}[]
\small
    \centering
    \begin{tabular}{|l|p{5cm}|}
    \hline
    \textbf{Model}  & \textbf{Optimal values} \\ \hline 
         Base &  --- \\ \hline
         Base + LM  & $\alpha=0.105, \beta= 0.497$ \\ \hline
         Base + WB  & $\gamma=7.09, \alpha=0.29,\beta=0.695$\\ \hline
         Base + WB\textsuperscript{ctx}  & $\gamma =2.697,\alpha=0.3521,\beta=0.789,\lambda=1.24$ \\ \hline
         Ours, $C=1$  & $\gamma=12.31, \delta: 8.25,\lambda=1.01,\alpha=0.889,\beta=0.14,\sigma=10.7,K=17 $ \\ \hline
         Ours, $\sigma=0$   &$\gamma=9.74,\delta=13.124,\lambda=1.77,\alpha=0.33,\beta=0.632,K=34,C=0.9918$ \\ \hline
    \end{tabular}
    \caption{Optimal hyper-parameters for all baseline models and other variants of our model.}
    \label{tab:hyper}
\end{table}
\subsection{Dataset creation details}
Adding to description in Section~\ref{sec:data}, we manually drive a robotic agent in 5 different rooms in the simulator~\cite{talbot2020benchbot} to obtain the images. We pre-process the images by generating captions using~\citep{yang2017dense}, followed by running the bias-target prediction Bi-LSTM model. Two volunteers from our organization agreed to write the instructions. We asked the volunteers to look at both the given image and the pre-processed biasing words and write instructions for the robot that includes one or more of the objects in the biasing words. We manually checked and removed any instruction that doesn't contain at least one word from the biasing word list and thus ensured the context is always valid. For recording, we have given the instructions (without image/biasing lists) to three volunteers, different from the ones who wrote the instructions, and asked them to record the instructions using their mobile phones. We have collected and converted all recordings to 16KHz wav format. We have not excluded any recordings from the collected set. Additionally, we have used two TTS models to generate recordings, as described in Section~\ref{sec:data}.
\balance
